# Supplementary material for: Knowing-how & Knowing-that: A New Task for Machine Comprehension of User Manuals
Source: arXiv:2306.04187 source file (2023-08-09)
Supplement: Supplementary file 1 [file appendix.tex]

% \appendix
% % \section{Data analysis}
% % \label{sec:da}
% % \input{tables-old/statis}
% \section{Semantic labels aligned to \kh and \kt}
% \label{sec:align}
% \begin{table}[]
%     \centering
% \begin{tabular}{|l|l|}
% \hline
% \multicolumn{1}{|c|}{Tags of ours}             & Tags in SemEval2016 \\ \hline
% \multicolumn{1}{|c|}{\multirow{2}{*}{subject}} & EXP                 \\ \cline{2-2} 
% \multicolumn{1}{|c|}{}                         & AGT                 \\ \hline
% \multicolumn{1}{|c|}{\multirow{4}{*}{object}}  & PAT                 \\ \cline{2-2} 
% \multicolumn{1}{|c|}{}                         & CONT                \\ \cline{2-2} 
% \multicolumn{1}{|c|}{}                         & DATV                \\ \cline{2-2} 
% \multicolumn{1}{|c|}{}                         & LINK                \\ \hline
% time                                           & TIME                \\ \hline
% location                                       & LOC                 \\ \hline
% \multirow{3}{*}{manner}                        & MANN                \\ \cline{2-2} 
%                                               & MATL                \\ \cline{2-2} 
%                                               & TOOL                \\ \hline
% \multirow{2}{*}{action\_state}                 & mNEG                \\ \cline{2-2} 
%                                               & mDEPD               \\ \hline
% \end{tabular}
%     \caption{Semantic labels aligned to \kh}
%     \label{tab:alig_kh}
% \end{table}
% \begin{table}[]
%     \centering
% \begin{tabular}{|l|l|}
% \hline
% \multicolumn{1}{|c|}{Tags of ours}              & Tags in SemEval2016   \\ \hline
% \multicolumn{1}{|c|}{\multirow{2}{*}{entity}}   & EXP                   \\ \cline{2-2} 
% \multicolumn{1}{|c|}{}                          & AGT                   \\ \hline
% sub-entity                                      & \multirow{2}{*}{FEAT} \\ \cline{1-1}
% property                                        &                       \\ \hline
% property                                        & Belg                  \\ \hline
% property\_value                                 & Clas                  \\ \hline
% \multicolumn{1}{|c|}{\multirow{4}{*}{patients}} & PAT                   \\ \cline{2-2} 
% \multicolumn{1}{|c|}{}                          & CONT                  \\ \cline{2-2} 
% \multicolumn{1}{|c|}{}                          & DATV                  \\ \cline{2-2} 
% \multicolumn{1}{|c|}{}                          & LINK                  \\ \hline
% time                                            & TIME                  \\ \hline
% location                                        & LOC                   \\ \hline
% \multirow{3}{*}{manner}                         & MANN                  \\ \cline{2-2} 
%                                                 & MATL                  \\ \cline{2-2} 
%                                                 & TOOL                  \\ \hline
% cause                                           & REAS                  \\ \hline
% \multirow{2}{*}{action\_state}                  & mNEG                  \\ \cline{2-2} 
%                                                 & mDEPD                 \\ \hline
% \end{tabular}
%     \caption{Semantic labels aligned to \kt}
%     \label{tab:alig_kt}
% \end{table}
% \section{Visualization of the proposed pipeline framework}
% \label{sec:pipe}

\appendix
\section{Details of Experiment \Rmnum{2}}
\textbf{LexicalMatching}
\begin{itemize}
    \item \textbf{BLEU}: Traditional Bleu considers the co-occurrence of n-grams between candidate and reference and adds a penalty factor of candidate answer length. To adjust it to fit our dataset better and inspired by previous work \cite{alfonseca2001prototype, yang2018adaptations}, when calculating n-gram co-occurrence, we first increase the co-occurrence score by providing higher scores for candidate answers containing keywords in the question. The keywords extraction API of the iFLYTEK open platform is used for our question keywords extraction. At the same time, we adjust parameter B in the BP penalty to better conform to our data set. The modified calculation formula is as follows:\\
    \begin{equation}
        P(n)=\frac{\sum_{ngrams}^{}C_{clip}(ngram)+C_{k}(r,c)}{\sum_{ngrams}^{}C(ngram)+C_{k}(r,c)}
    \end{equation}
    \begin{equation}
    BP = \left\{\begin{matrix}
1, & if \quad \left |c  \right | \geqslant B\ast \left |r  \right |\\ 
e^{\left (1-B\ast \left |r  \right | / \left |c  \right | \right )}, & if \quad \left |c  \right | < B\ast \left |r  \right |
\end{matrix}\right. 
    \end{equation}
    \begin{equation}
        BLEU=BP\cdot exp(\sum_{n=1}^{N} W_{n}logP(n))
    \end{equation}
    where $r$ represents question text, $c$ represents the candidate answer, $C_{k}$ represents how many keywords of question appear in the candidate answer, $\left |r  \right |$ and $\left |c  \right |$ represents the length of question text and candidate answer. We set B to 3 to better match our data set.
    \item \textbf{Levenshtein Distance}: For Levenshtein Distance, we use the transformation shown in Formula 1 to calculate the lexical similarity between question and candidate answers.
\end{itemize}
\hfill\break
\textbf{SemanticMatching}
The focus of the models based on Semantic Matching is to calculate the semantic similarity between the question text and all candidate answers. And then we select the top n with the highest score as the final answer. For the following models, we choose the top 2 sentences in the score ranking as the answers.
\begin{itemize}
    \item \textbf{Bert Base}: We take the average of the output vector corresponding to each token as the representation of the whole sentence, and use the cosine similarity to calculate the distance between two vectors.
    \item \textbf{Char CNN}: We first use LTP to segment the sentence, and then query the vector of corresponding tokens in the vocabulary. If the vector for one token cannot be found in the vocabulary, we further divide the token into a shorter sequence, and then query in the vocabulary again, until it is divided into a single word. Finally, the average of all word vectors in the sentence is taken as the representation of the sentence, and the cosine similarity is used to calculate the distance between the two vectors.
    \item \textbf{Chinese Word Vectors}: Same calculation method as Char CNN.
    \item \textbf{Bert Score}: We directly call the API in the GitHub project to calculate the similarity between two sentences\cite{bert-score}.
\end{itemize}
\hfill\break
\textbf{KeywordsMatching}
We use the TF-IDF algorithm to extract keywords from each document, and the top 10 keywords are obtained for each document. At the same time, we use the keywords extraction API of the iFLYTEK open platform to obtain the keywords of the question text.
\begin{itemize}
    \item \textbf{Synonyms Plus}: We choose the sentence rewriting API of the iFLYTEK open platform for question rewriting. For synonyms replacement, we use the Chinese word2vec pre-training vectors to find the top 10 words with the highest cosine similarity in the thesaurus as synonyms of the target word. When matching the keywords between questions and answers, we use three indicators: exact match, synonym matching, and cosine similarity based on bert encoding, and give them weights of 0.9, 0.7, and 0.6 respectively to calculate the final score.
    \item \textbf{Keywords Window}: We calculate the matching score between each candidate answer and question according to the following formula:
    \begin{equation}
    \begin{split}
    score=16\ast question\_keywords+ \\ 16\ast answer\_keywords+ \\ 16\ast matched\_keywords+ \\ 16\ast same\_parse\_subtree\_score- \\ 4\ast \sqrt{keywords\_distance}
    \end{split}
    \end{equation}
    where $question\_keywords$ represents the number of candidate answer keywords existing in the question text, $answer\_keywords$ represents the number of question keywords existing in the candidate answers, $matched\_keywords$ represents the number of words that are both question keywords and answer keywords, $same\_parse\_subtree\_score$ represents how many question keywords are on the same sub\_tree of the candidate answer parsing tree, $keywords\_distance$ represents the distance between the two question keywords that are farthest apart in the candidate answer text.
\end{itemize}
\hfill\break
\textbf{Pre-trainingLanguageModel}
For pre-training language models, we splice the question text and the document and then input it to the model to get the start and end positions of the predicted answer span in the document to get the final answer. 

\hfill\break
\textbf{SelfSupervised}
We use the pre-training QA models on hugging face for fine-tuning. The same splicing method as the pre-training stage is used to construct the input data. We choose the AdamW\cite{loshchilov2017decoupled} as the optimizer, the learning rate is set to 1e-5, and a total of three epochs are trained.

\hfill\break
\textbf{Fine-tuning on Pre-training Model}
We conduct additional experiments on fine-tuning models. We divide the annotated QA data set into two parts, half of which is used for fine-tuning the model, and the remaining half of the data is used for evaluation. To ensure that the model can predict multiple spans at one time and compare with other models fairly, we splice the question text and candidate sentence into the model each time and output whether the sentence is the answer to the question. Finally, we take all the sentences that the model considers to be the answer as the final result. 

% \section{Supplement to Experiment \Rmnum{2} for different types of questions}
% \input{tables-old/QA_factoid.tex}
% \input{tables-old/QA_procedure.tex}
% \input{tables-old/QA_inconsistency.tex}

% \input{tables-old/QA_fine-tune_PLM.tex}

\section{Illustration Supplements}
  \begin{figure*}[t]
    \centering
    \includegraphics[width=\textwidth]{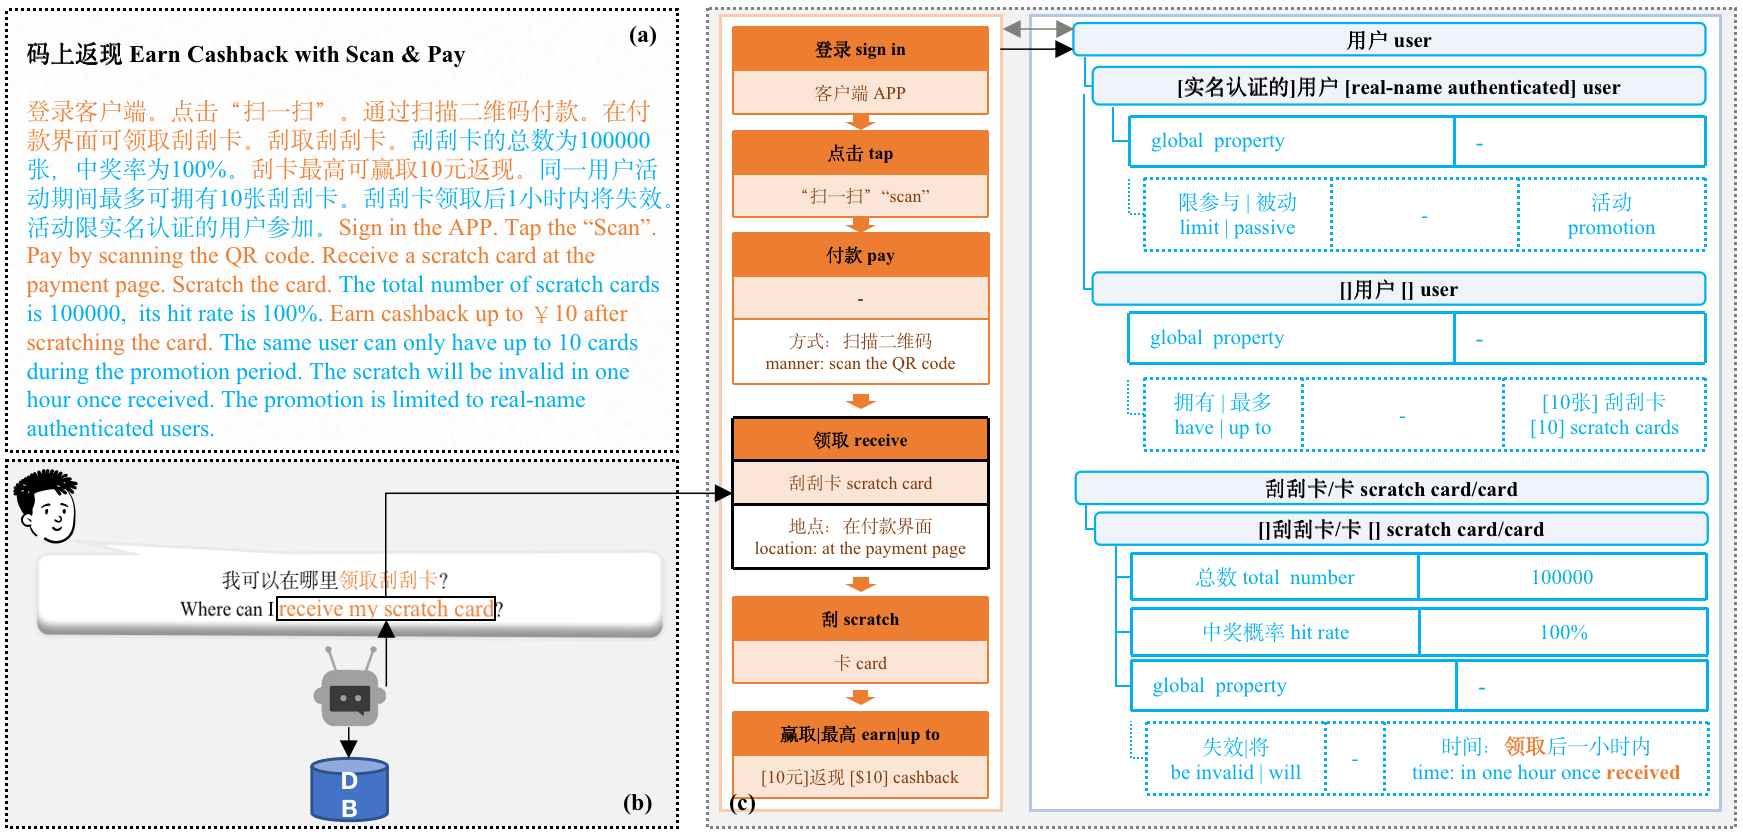}
    \caption{Illustration of a user instruction~(a), a factoid-style question~(b), and the annotated user instruction~(c), whose \textcolor{orange}{left part} is the sequence of steps, \textcolor{cyan}{right part} contains the set of entities.
    }
    % \vspace{-0.6cm}
    \label{fig:example_factoid}
\end{figure*}
  \begin{figure*}[t]
    \centering
    \includegraphics[width=\textwidth]{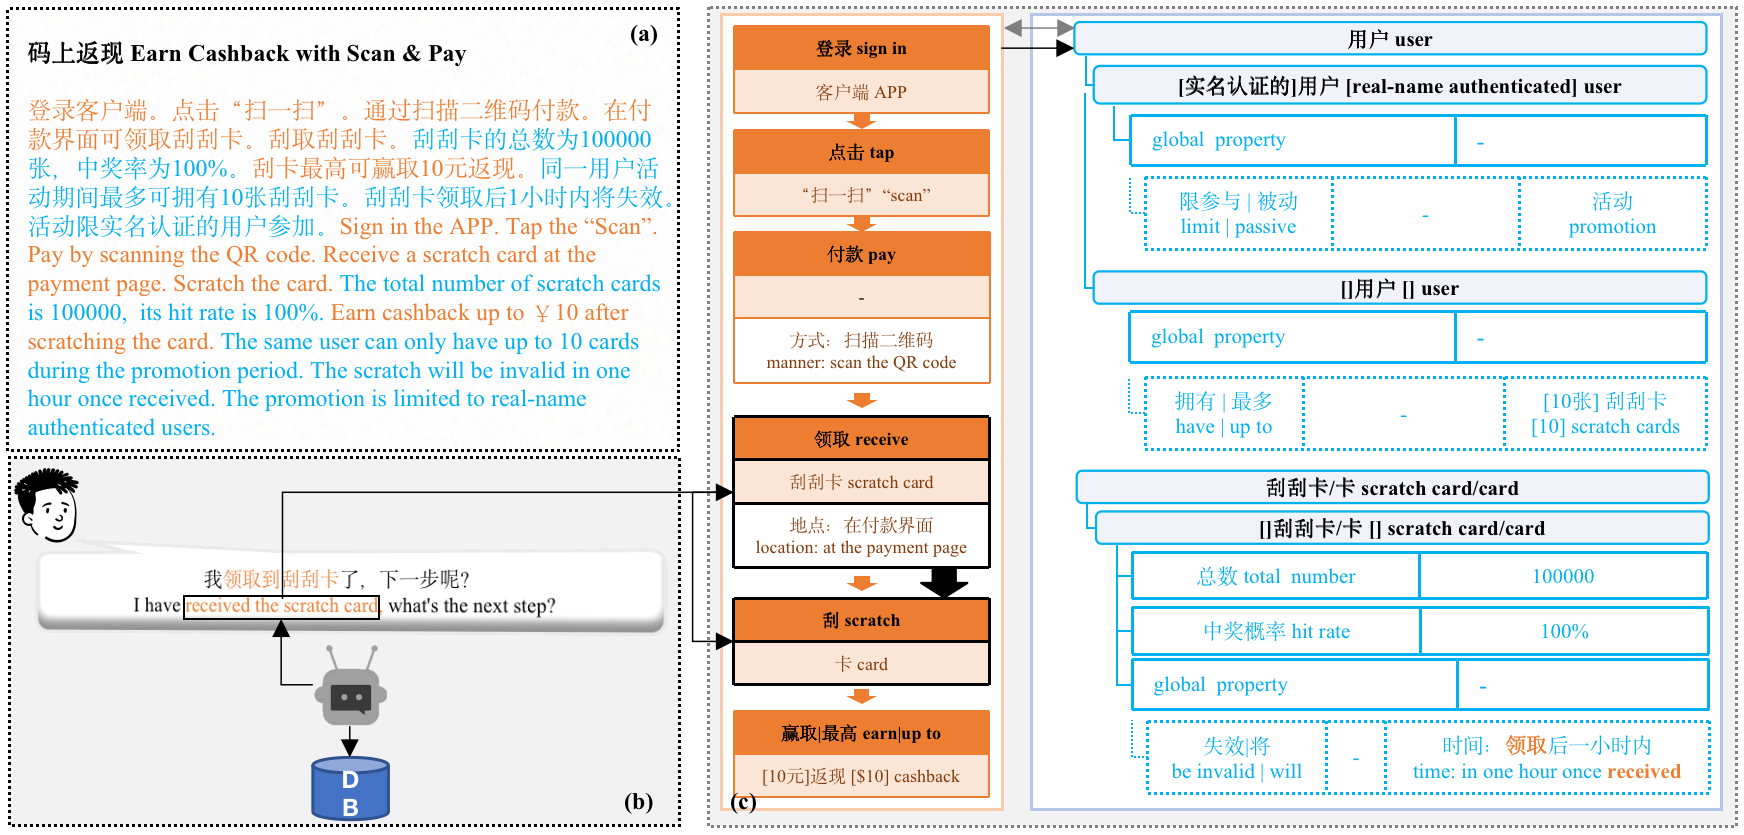}
    \caption{Illustration of a user instruction~(a), a procedure-style question~(b), and the annotated user instruction~(c), whose \textcolor{orange}{left part} is the sequence of steps, \textcolor{cyan}{right part} contains the set of entities.
    }
    % \vspace{-0.6cm}
    \label{fig:example_procedure}
\end{figure*}

\section{QA Example}

\begin{figure*}[t]
    \centering
    \includegraphics[width=\textwidth]{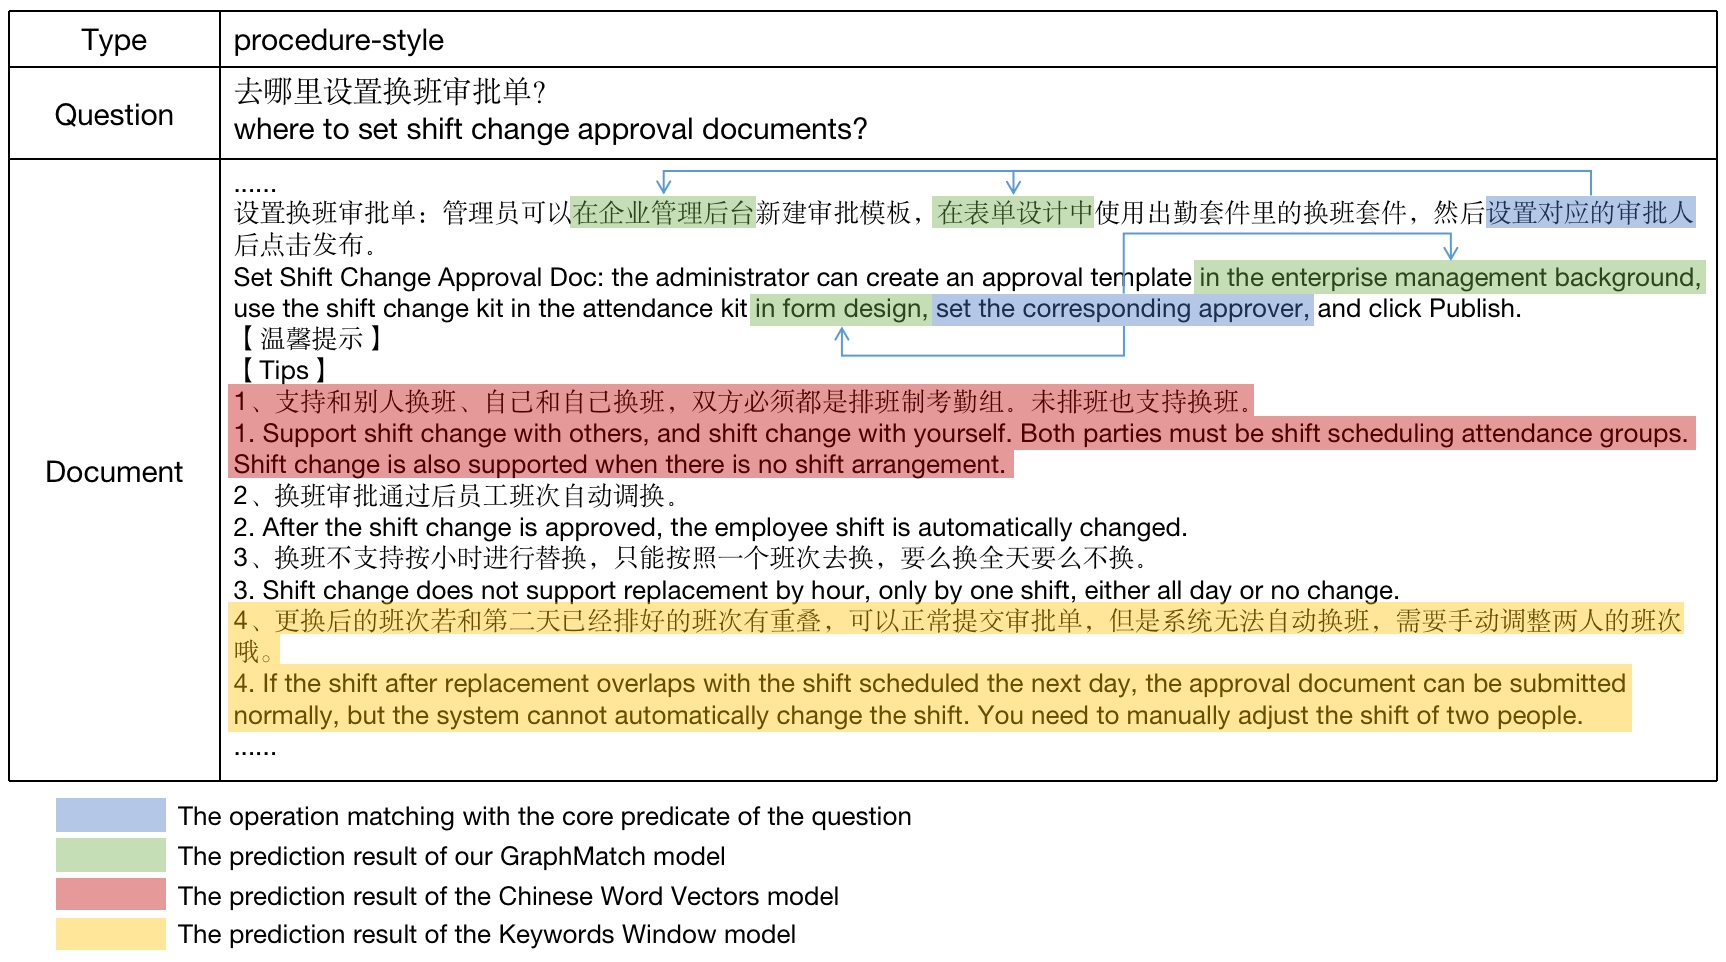}
    % \label{fig:example_factoid}
    \caption{Examples of Question Answering for different types of questions. The \colorbox[RGB]{180,199,231}{blue} part represents the operation matching with the core predicate of the question. The \colorbox[RGB]{230,153,153}{red} part is the prediction result of the Chinese Word Vectors model. The \colorbox[RGB]{255,230,153}{yellow} part is the prediction result of the Keywords Window model. The \colorbox[RGB]{198,222,181}{green} part is the prediction result of our HUM model.}
\end{figure*}
\begin{figure*}[t]
    \centering
    \includegraphics[width=\textwidth]{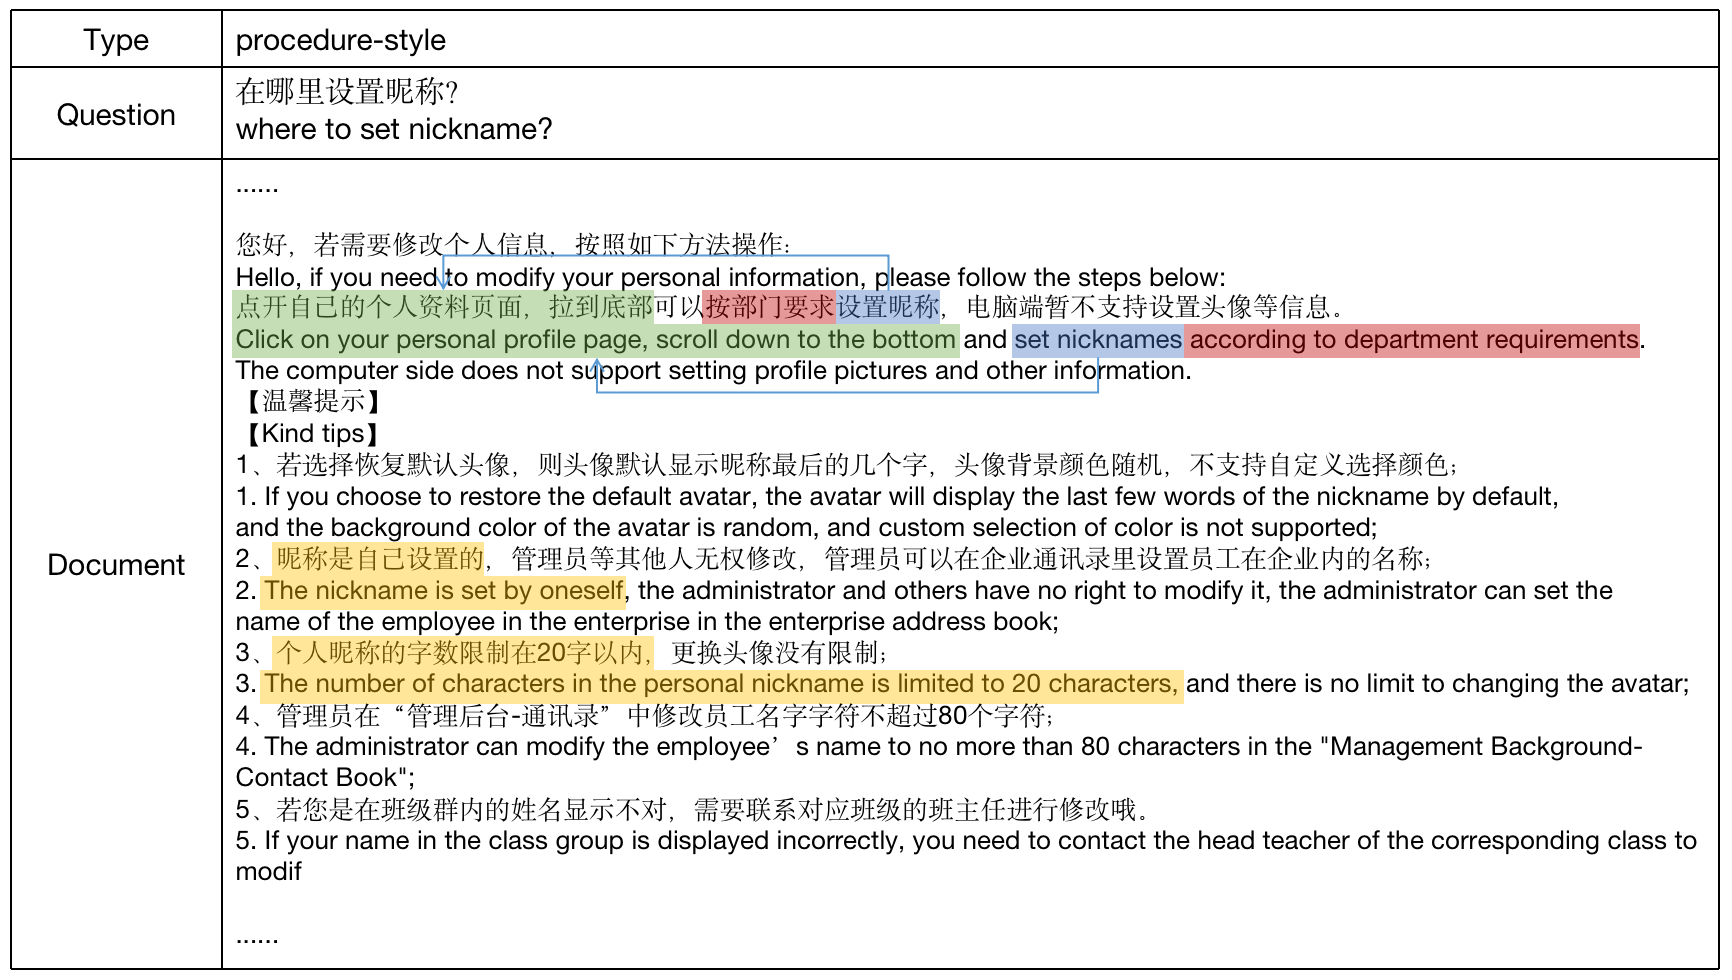}
    % \label{fig:example_factoid}
\end{figure*}
\begin{figure*}[t]
    \centering
    \includegraphics[width=\textwidth]{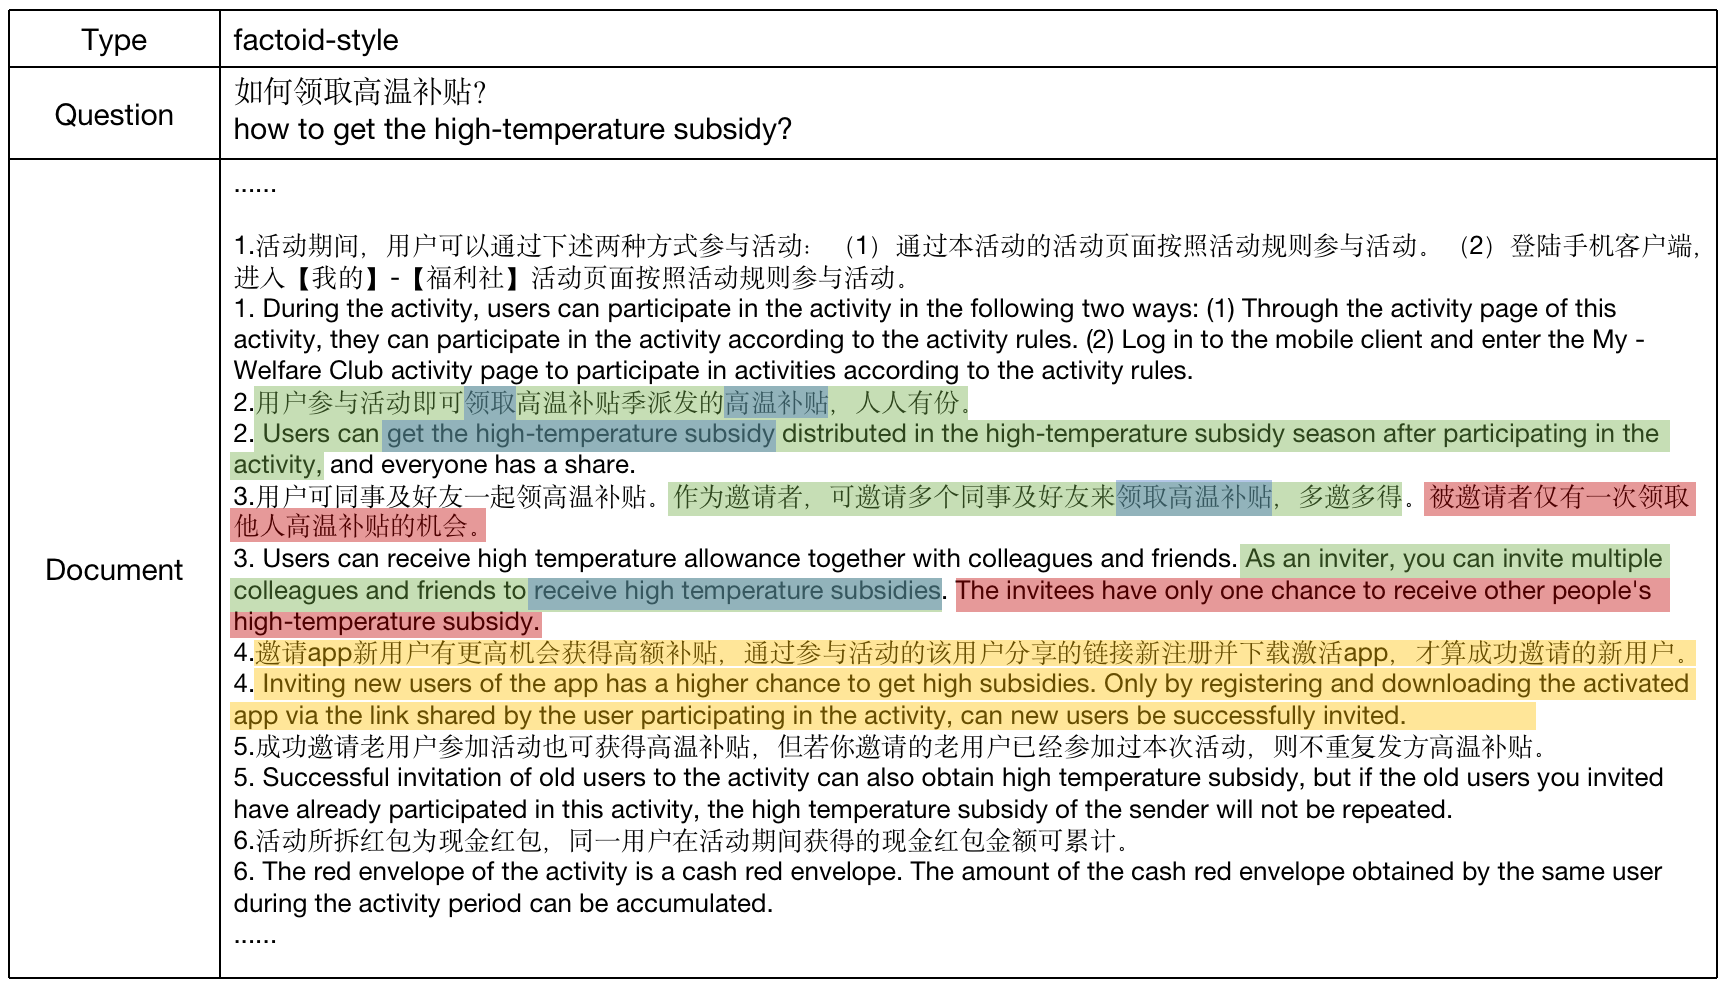}
    % \label{fig:example_factoid}
\end{figure*}
\begin{figure*}[t]
    \centering
    \includegraphics[width=\textwidth]{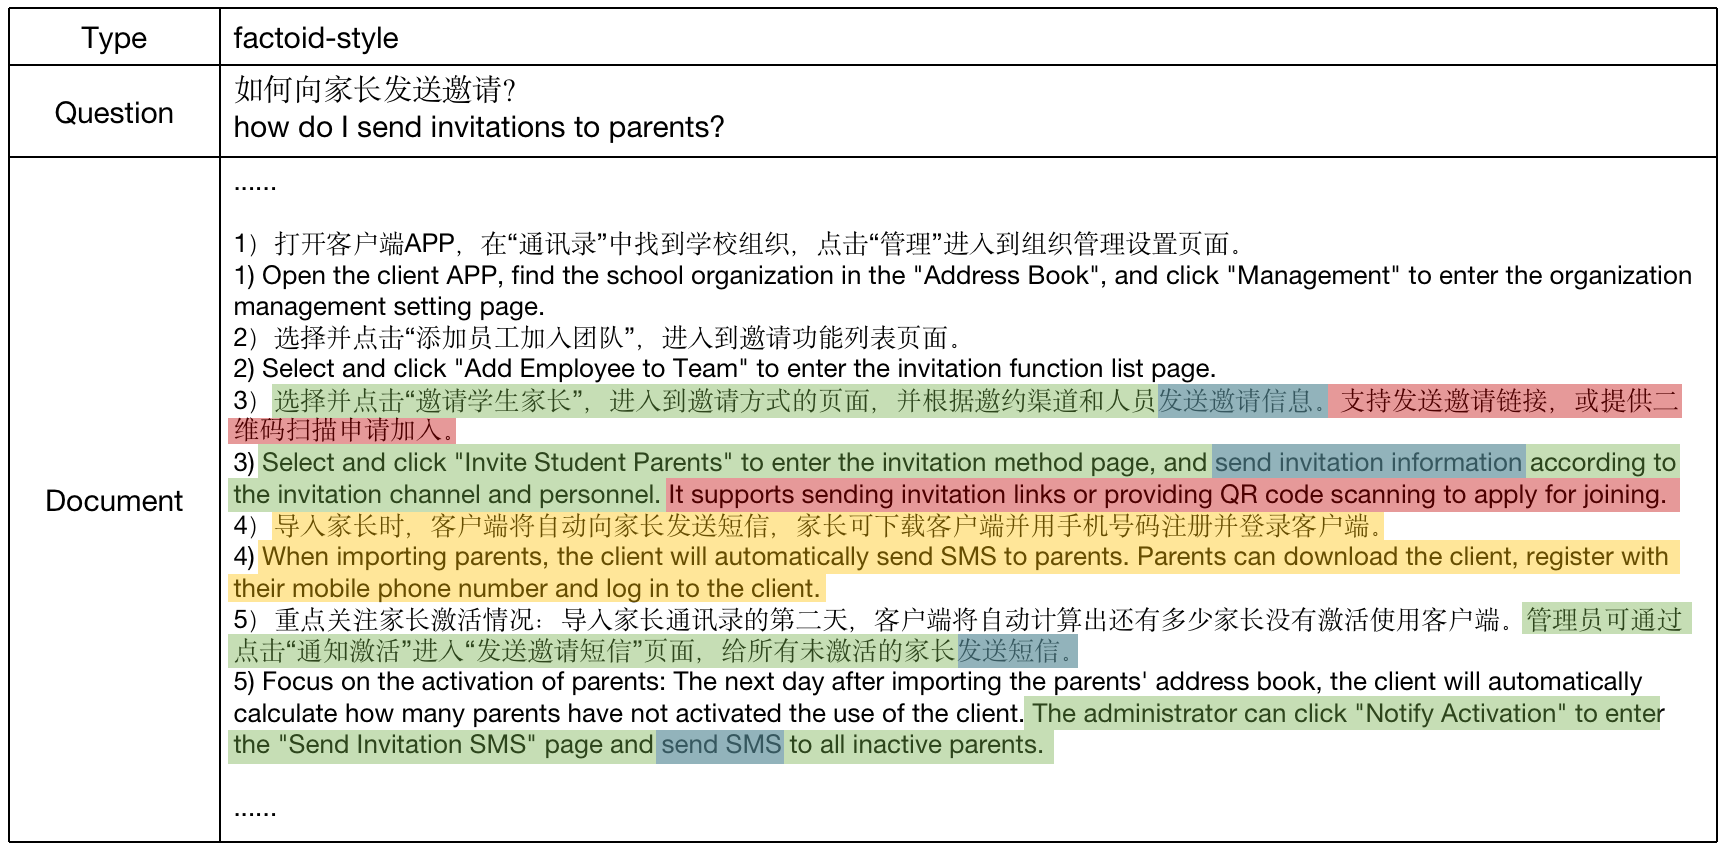}
    % \label{fig:example_factoid}
\end{figure*}
\begin{figure*}[t]
    \centering
    \includegraphics[width=\textwidth]{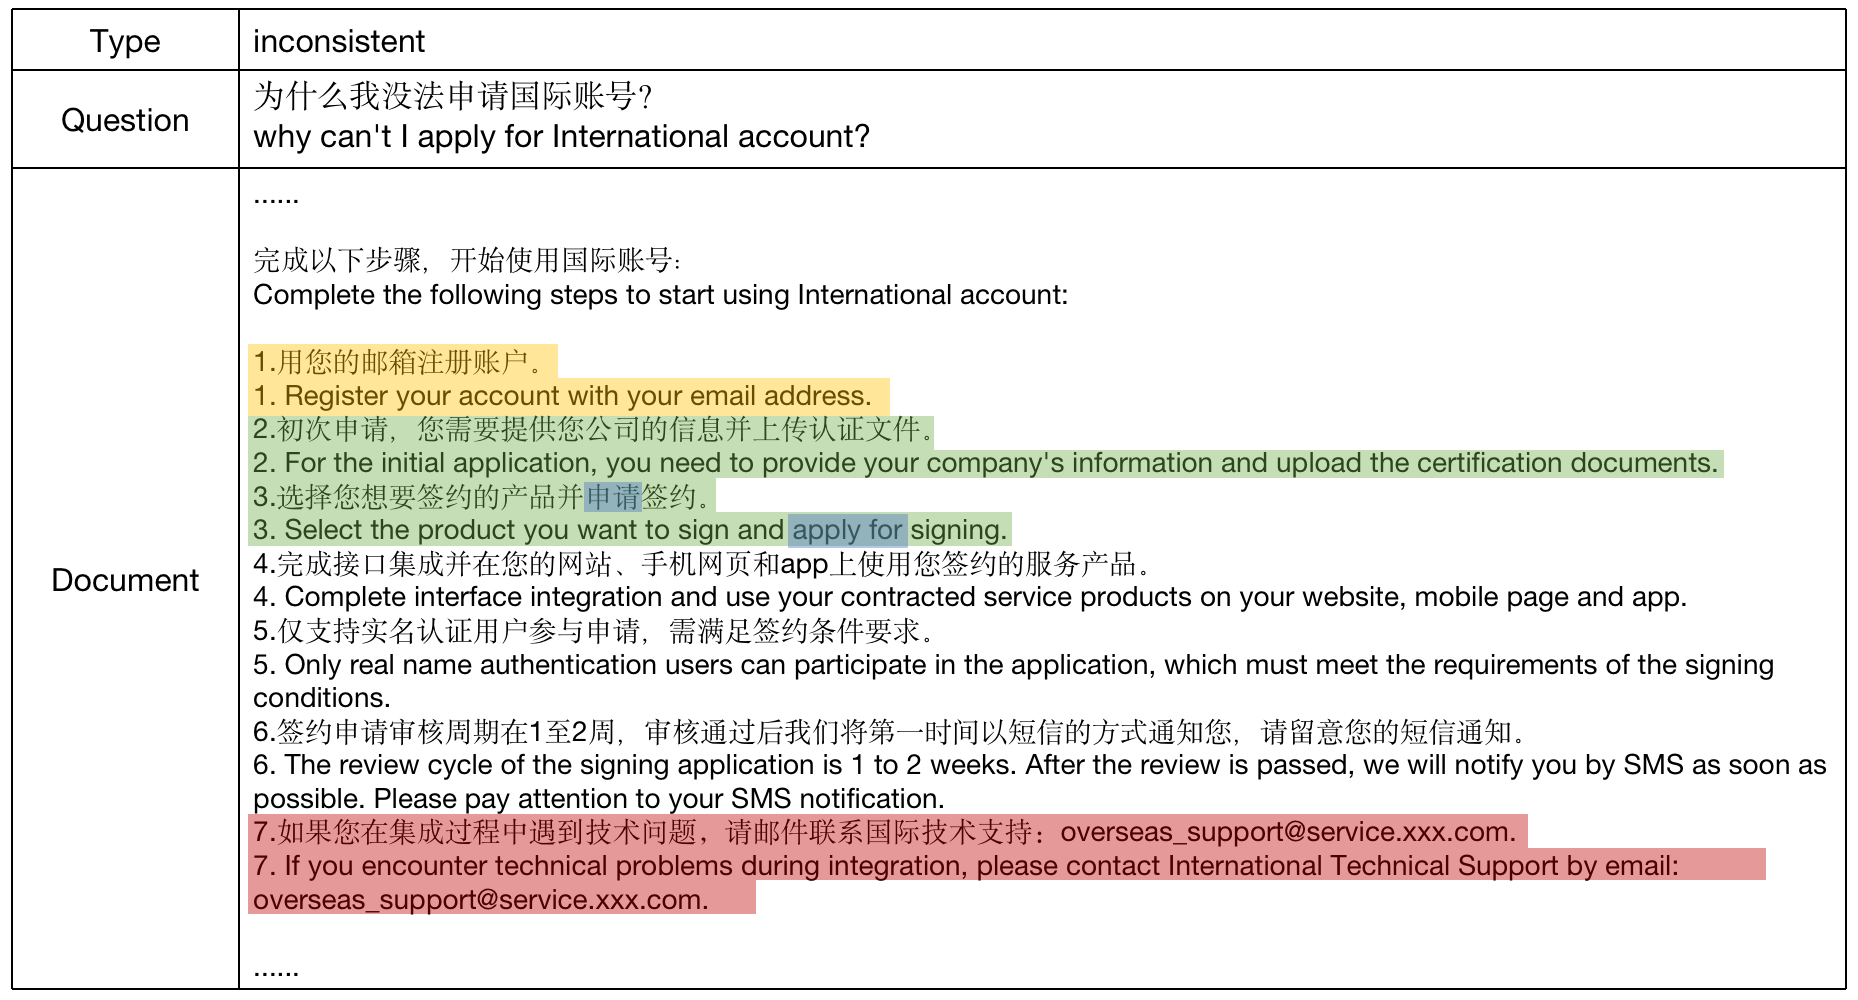}
    % \label{fig:example_factoid}
\end{figure*}
\begin{figure*}[t]
    \centering
    \includegraphics[width=\textwidth]{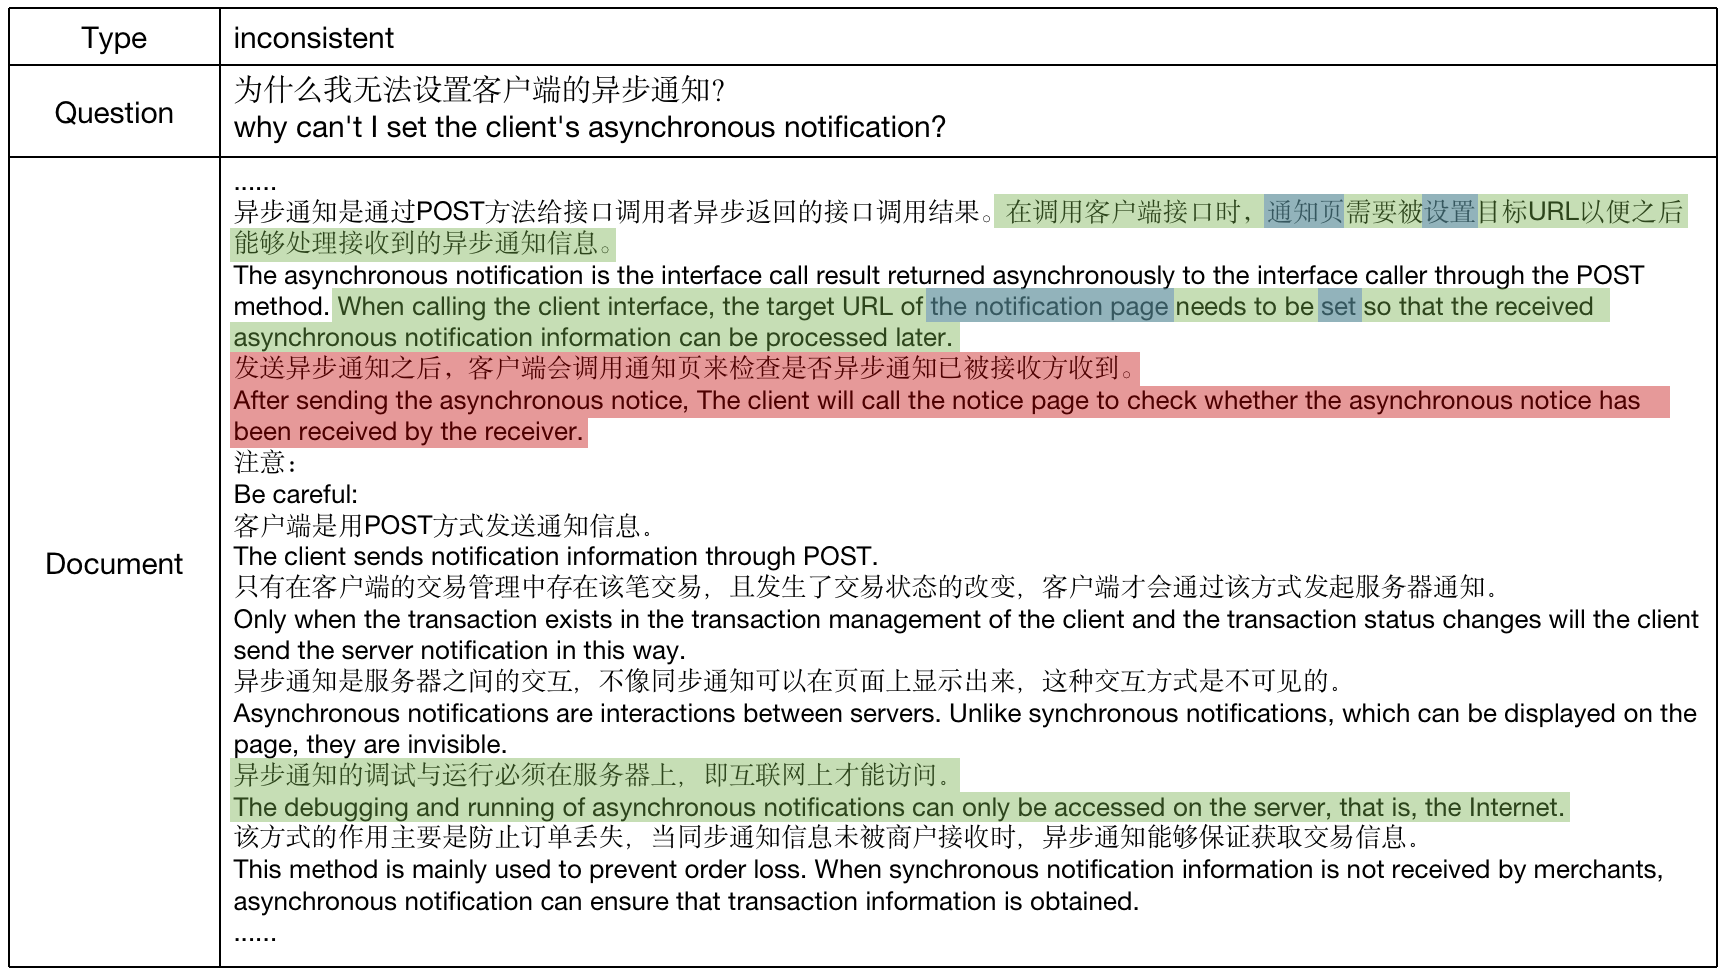}
    % \label{fig:example_factoid}
\end{figure*}
